# Supplementary material for: A tale of two theories of gravity in asymptotically Anti-de Sitter spacetime
Source: arXiv:2210.10154 source file (2022-10-25)
Supplement: Supplementary file 1 [file Supplement.pdf]

# Supplement of "A tale of two theories of gravity in asymptotically Anti-de Sitter spacetime"

by Remigiusz Durka and Jerzy Kowalski-Glikman

Bellow we collect the asymptotic expressions for the relevant geometric objects necessary for the computations within the asymptotic AdS framework.

## 1 Tetrads

Asymptotic expansion of the metric $g_{\mu\nu} = \bar{g}_{\mu\nu} + g^{(1)}_{\mu\nu}$, where

$$g^{(1)}_{\mu\nu} = \begin{pmatrix} \frac{h_{tt}[t,\theta,\phi]}{r} & \frac{h_{tr}[t,\theta,\phi]}{r^4} & \frac{h_{t\theta}[t,\theta,\phi]}{r} & \frac{h_{t\phi}[t,\theta,\phi]}{r} \\ \frac{h_{tr}[t,\theta,\phi]}{r^4} & \frac{h_{rr}[t,\theta,\phi]}{r^5} & \frac{h_{r\theta}[t,\theta,\phi]}{r^4} & \frac{h_{r\phi}[t,\theta,\phi]}{r^4} \\ \frac{h_{t\theta}[t,\theta,\phi]}{r} & \frac{h_{r\theta}[t,\theta,\phi]}{r^4} & \frac{h_{\theta\theta}[t,\theta,\phi]}{r} & \frac{h_{\theta\phi}[t,\theta,\phi]}{r} \\ \frac{h_{t\phi}[t,\theta,\phi]}{r} & \frac{h_{r\phi}[t,\theta,\phi]}{r^4} & \frac{h_{\theta\phi}[t,\theta,\phi]}{r} & \frac{h_{\phi\phi}[t,\theta,\phi]}{r} \end{pmatrix} \tag{1.1}$$

leads to tetrad expansion:

$$e^a = \bar{e}^a + e^{(1)a}\,, \tag{1.2}$$

where AdS tetrads are

$$\bar{e}^0 = \sqrt{1 - \frac{\Lambda r^2}{3}}dt, \quad \bar{e}^1 = \frac{1}{\sqrt{1 - \frac{\Lambda r^2}{3}}}dr, \quad \bar{e}^2 = rd\theta, \quad \bar{e}^3 = r\sin\theta d\phi\,, \tag{1.3}$$

and for which (in torsionless case) we easily obtain the AdS spin connections

$$\begin{aligned} \bar{\omega}^{01} &= -\frac{\Lambda}{3} r dt & \bar{\omega}^{23} &= -\cos\theta d\varphi \\ \bar{\omega}^{12} &= -\sqrt{1 - \frac{\Lambda}{3}r^2}d\theta & \bar{\omega}^{13} &= -\sqrt{1 - \frac{\Lambda}{3}r^2}\sin\theta d\varphi\,. \end{aligned} \tag{1.4}$$

The tetrads $e^{(1)a}$ can be written explicitly as:

$$\begin{aligned} e^{(1)0} &= -\frac{1}{2}\sqrt{-\frac{3}{\Lambda}}\left(\frac{h_{tt}[t,\theta,\phi]}{r^2}dt + \frac{h_{tr}[t,\theta,\phi]}{r^5}dr + \frac{h_{t\theta}[t,\theta,\phi]}{r^2}d\theta + \frac{h_{t\phi}[t,\theta,\phi]}{r^2}d\phi\right) \\ e^{(1)1} &= \frac{1}{2}\sqrt{-\frac{\Lambda}{3}}\left(\frac{h_{tr}[t,\theta,\phi]}{r^3}dt + \frac{h_{rr}[t,\theta,\phi]}{r^4}dr + \frac{h_{r\theta}[t,\theta,\phi]}{r^3}d\theta + \frac{h_{r\phi}[t,\theta,\phi]}{r^3}d\phi\right) \\ e^{(1)2} &= \frac{1}{2}\left(\frac{h_{t\theta}[t,\theta,\phi]}{r^2}dt + \frac{h_{r\theta}[t,\theta,\phi]}{r^5}dr + \frac{h_{\theta\theta}[t,\theta,\phi]}{r^2}d\theta + \frac{h_{\theta\phi}[t,\theta,\phi]}{r^2}d\phi\right) \\ e^{(1)3} &= \frac{1}{2}\frac{1}{\sin\theta}\left(\frac{h_{t\phi}[t,\theta,\phi]}{r^2}dt + \frac{h_{r\phi}[t,\theta,\phi]}{r^5}dr + \frac{h_{\theta\phi}[t,\theta,\phi]}{r^2}d\theta + \frac{h_{\phi\phi}[t,\theta,\phi]}{r^2}d\phi\right)\,. \end{aligned} \tag{1.5}$$

## 2 Asymptotic Christoffel symbols

Similarly to the asymptotic expansion of the metric $g_{\mu\nu} = \bar{g}_{\mu\nu} + g^{(1)}_{\mu\nu}$ we have the asymptotic expansion of Christoffel symbols

$$\Gamma^{\mu}{}_{\nu\rho} = \bar{\Gamma}^{\mu}{}_{\nu\rho} + \Gamma^{(1)\mu}{}_{\nu\rho}\,, \tag{2.1}$$

where the AdS part is

$$\begin{aligned}
\bar{\Gamma}^{t}{}_{r,t} &= \frac{r\Lambda}{(r^2\Lambda - 3)} \\
\bar{\Gamma}^{r}{}_{t,t} &= \frac{1}{9}\, r\left(r^2\Lambda - 3\right) \\
\bar{\Gamma}^{r}{}_{r,r} &= -\frac{r\Lambda}{(r^2\Lambda - 3)} \\
\bar{\Gamma}^{r}{}_{\theta,\theta} &= \frac{1}{3}\, r\left(r^2\Lambda - 3\right) \\
\bar{\Gamma}^{\theta}{}_{\theta,r} &= \frac{1}{r} \\
\bar{\Gamma}^{\varphi}{}_{\varphi,r} &= \frac{1}{r}
\end{aligned}$$

and the perturbation part corresponds to

$$\begin{aligned}
\Gamma^{(1)t}{}_{t,t} &= \frac{1}{r^3}\left(\frac{3}{2\Lambda}\partial_t h_{tt} - \frac{1}{3}\Lambda\right) h_{tr} \\
\Gamma^{(1)t}{}_{r,t} &= -\frac{9}{2r^4\Lambda} h_{tt} \\
\Gamma^{(1)t}{}_{r,r} &= -\frac{3}{2r^7\Lambda}\left(6h_{tr} + \partial_t h_{rr}\right) \\
\Gamma^{(1)t}{}_{\theta,t} &= \frac{3}{2r^3\Lambda}\partial_r h_{tt} \\
\Gamma^{(1)t}{}_{\theta,r} &= -\frac{9}{2r^4\Lambda} h_{t\theta}
\end{aligned}$$

$$\Gamma^{(1)t}{}_{t,t} = \frac{\frac{9\partial_t h_{\rm tt}}{\Lambda} - 2\Lambda h_{\rm tr}}{6r^3}$$

$$\Gamma^{(1)t}{}_{r,t} = -\frac{9h_{\rm tt}}{2r^4\Lambda}$$

$$\Gamma^{(1)t}{}_{r,r} = -\frac{3\left(6h_{\rm tr} + \partial_t h_{\rm rr}\right)}{2r^7\Lambda}$$

$$\Gamma^{(1)t}{}_{\theta,t} = \frac{3\partial_\theta h_{\rm tt}}{2r^3\Lambda}$$

$$\Gamma^{(1)t}{}_{\theta,r} = -\frac{9h_{\rm t\theta}}{2r^4\Lambda}$$

$$\Gamma^{(1)t}{}_{\theta,\theta} = -\frac{2\Lambda h_{\rm tr} - 6\partial_\theta h_{\rm t\theta} + 3\partial_t h_{\theta\theta}}{2r^3\Lambda}$$

$$\Gamma^{(1)t}{}_{\varphi,t} = \frac{3\partial_\varphi h_{\rm tt}}{2r^3\Lambda}$$

$$\Gamma^{(1)t}{}_{\varphi,r} = -\frac{9h_{\rm t\varphi}}{2r^4\Lambda}$$

$$\Gamma^{(1)t}{}_{\varphi,\theta} = \frac{3\left(-2\cot(\theta)h_{\rm t\varphi} + \partial_\varphi h_{\rm t\theta} + \partial_\theta h_{\rm t\varphi} - \partial_t h_{\theta\varphi}\right)}{2r^3\Lambda}$$

$$\Gamma^{(1)t}{}_{\varphi,\varphi} = \frac{-2\Lambda h_{\rm tr}\sin^2(\theta) + 6\cos(\theta)h_{\rm t\theta}\sin(\theta) + 6\partial_\varphi h_{\rm t\varphi} - 3\partial_t h_{\varphi\varphi}}{2r^3\Lambda}$$

$$\Gamma^{(1)r}{}_{t,t} = \frac{1}{54}\Lambda\left(2\Lambda^2 h_{\rm rr} - 9h_{\rm tt}\right)$$

$$\Gamma^{(1)r}{}_{r,t} = \frac{\Lambda\left(2h_{\rm tr} - \partial_t h_{\rm rr}\right)}{6r^3}$$

$$\Gamma^{(1)r}{}_{r,r} = \frac{\Lambda h_{\rm rr}}{2r^4}$$

$$\Gamma^{(1)r}{}_{\theta,t} = -\frac{1}{6}\Lambda h_{\rm t\theta}$$

$$\Gamma^{(1)r}{}_{\theta,r} = \frac{\Lambda\left(2h_{\rm r\theta} - \partial_\theta h_{\rm rr}\right)}{6r^3}$$

$$\Gamma^{(1)r}{}_{\theta,\theta} = \frac{1}{18}\Lambda\left(2\Lambda h_{\rm rr} - 3h_{\theta\theta}\right)$$

$$\Gamma^{(1)r}{}_{\varphi,t} = -\frac{1}{6}\Lambda h_{\rm t\varphi}$$

$$\Gamma^{(1)r}{}_{\varphi,r} = \frac{\Lambda\left(2h_{\rm r\varphi} - \partial_\varphi h_{\rm rr}\right)}{6r^3}$$

$$\Gamma^{(1)r}{}_{\varphi,\theta} = -\frac{1}{6}\Lambda h_{\theta\varphi}$$

$$\Gamma^{(1)r}{}_{\varphi,\varphi} = \frac{1}{18}\Lambda\left(2\Lambda\sin^2(\theta)h_{\rm rr} - 3h_{\varphi\varphi}\right)$$

and

$$\Gamma^{(1)\theta}{}_{t,t} = -\frac{2h_{\mathrm{r}\theta}\Lambda^2 + 9\partial_\theta h_{\mathrm{tt}} - 18\partial_t h_{\mathrm{t}\theta}}{18r^3}$$
$$\Gamma^{(1)\theta}{}_{r,t} = -\frac{3h_{\mathrm{t}\theta}}{2r^4}$$
$$\Gamma^{(1)\theta}{}_{r,r} = -\frac{6h_{\mathrm{r}\theta} + \partial_\theta h_{\mathrm{rr}}}{2r^7}$$
$$\Gamma^{(1)\theta}{}_{\theta,t} = \frac{\partial_t h_{\theta\theta}}{2r^3}$$
$$\Gamma^{(1)\theta}{}_{\theta,r} = -\frac{3h_{\theta\theta}}{2r^4}$$
$$\Gamma^{(1)\theta}{}_{\theta,\theta} = \frac{3\partial_\theta h_{\theta\theta} - 2\Lambda h_{\mathrm{r}\theta}}{6r^3}$$
$$\Gamma^{(1)\theta}{}_{\varphi,t} = \frac{\partial_\varphi h_{\mathrm{t}\theta} - \partial_\theta h_{\mathrm{t}\varphi} + \partial_t h_{\theta\varphi}}{2r^3}$$
$$\Gamma^{(1)\theta}{}_{\varphi,r} = -\frac{3h_{\theta\varphi}}{2r^4}$$
$$\Gamma^{(1)\theta}{}_{\varphi,\theta} = \frac{\partial_\varphi h_{\theta\theta} - 2\cot(\theta)h_{\theta\varphi}}{2r^3}$$
$$\Gamma^{(1)\theta}{}_{\varphi,\varphi} = \frac{-2\Lambda h_{\mathrm{r}\theta}\sin^2(\theta) + 6\cos(\theta)h_{\theta\theta}\sin(\theta) + 6\partial_\varphi h_{\theta\varphi} - 3\partial_\theta h_{\varphi\varphi}}{6r^3}$$
$$\Gamma^{(1)\varphi}{}_{t,t} = -\frac{\csc^2(\theta)\left(2h_{\mathrm{r}\varphi}\Lambda^2 + 9\left(\partial_\varphi h_{\mathrm{tt}} - 2\partial_t h_{\mathrm{t}\varphi}\right)\right)}{18r^3}$$
$$\Gamma^{(1)\varphi}{}_{r,t} = -\frac{3\csc^2(\theta)h_{\mathrm{t}\varphi}}{2r^4}$$
$$\Gamma^{(1)\varphi}{}_{r,r} = -\frac{\csc^2(\theta)\left(6h_{\mathrm{r}\varphi} + \partial_\varphi h_{\mathrm{rr}}\right)}{2r^7}$$
$$\Gamma^{(1)\varphi}{}_{\theta,t} = \frac{\csc^2(\theta)\left(-\partial_\varphi h_{\mathrm{t}\theta} + \partial_\theta h_{\mathrm{t}\varphi} + \partial_t h_{\theta\varphi}\right)}{2r^3}$$
$$\Gamma^{(1)\varphi}{}_{\theta,r} = -\frac{3\csc^2(\theta)h_{\theta\varphi}}{2r^4}$$
$$\Gamma^{(1)\varphi}{}_{\theta,\theta} = -\frac{\csc^2(\theta)\left(2\Lambda h_{\mathrm{r}\varphi} + 3\partial_\varphi h_{\theta\theta} - 6\partial_\theta h_{\theta\varphi}\right)}{6r^3}$$
$$\Gamma^{(1)\varphi}{}_{\varphi,t} = \frac{\csc^2(\theta)\partial_t h_{\varphi\varphi}}{2r^3}$$
$$\Gamma^{(1)\varphi}{}_{\varphi,r} = -\frac{3\csc^2(\theta)h_{\varphi\varphi}}{2r^4}$$
$$\Gamma^{(1)\varphi}{}_{\varphi,\theta} = \frac{\csc^2(\theta)\left(\partial_\theta h_{\varphi\varphi} - 2\cot(\theta)h_{\varphi\varphi}\right)}{2r^3}$$
$$\Gamma^{(1)\varphi}{}_{\varphi,\varphi} = \frac{3\partial_\varphi h_{\varphi\varphi}\csc^2(\theta) - 2\Lambda h_{\mathrm{r}\varphi} + 6\cot(\theta)h_{\theta\varphi}}{6r^3}$$

## 3 Asymptotic AdS-curvature components

The AdS curvature $F^{\lambda}{}_{\mu\sigma\nu} = R^{\lambda}{}_{\mu\sigma\nu} - \frac{\Lambda}{3}(g^{\lambda}{}_{\sigma} g_{\mu\nu} - g^{\lambda}{}_{\nu} g_{\mu\sigma})$ has the vanishing $\bar{F}$ part of the $F^{\lambda}{}_{\mu\sigma\nu} = \bar{F}^{\lambda}{}_{\mu\sigma\nu} + F^{(1)\,\lambda}{}_{\mu\sigma\nu}$ decomposition, and we write

$$F^{t}{}_{r,r,t} = \frac{1}{r^5}\left(\frac{9}{2\Lambda}h_{tt} - \frac{1}{6}\Lambda h_{\rm rr}\right)$$

$$F^{t}{}_{r,\theta,t} = \frac{\left(\Lambda^2 h_{\rm rr}{}^{(0,1,0)} + 27\left(h_{\rm t\theta}{}^{(1,0,0)} - h_{\rm tt}{}^{(0,1,0)}\right)\right)}{6\Lambda r^4}$$

$$F^{t}{}_{r,\theta,r} = -\frac{9h_{\rm t\theta}}{2\Lambda r^5}$$

$$F^{t}{}_{r,\varphi,t} = \frac{\left(\Lambda^2 h_{\rm rr}{}^{(0,0,1)} + 27\left(h_{\rm t\varphi}{}^{(1,0,0)} - h_{\rm tt}{}^{(0,0,1)}\right)\right)}{6\Lambda r^4}$$

$$F^{t}{}_{r,\varphi,r} = -\frac{9h_{\rm t\varphi}}{2\Lambda r^5}$$

$$F^{t}{}_{r,\varphi,\theta} = -\frac{9\left(h_{\rm t\theta}{}^{(0,0,1)} - h_{\rm t\varphi}{}^{(0,1,0)}\right)}{2\Lambda r^4}$$

$$F^{t}{}_{\theta,r,t} = \frac{\left(\Lambda^2 h_{\rm rr}{}^{(0,1,0)} + 27\left(h_{\rm t\theta}{}^{(1,0,0)} - h_{\rm tt}{}^{(0,1,0)}\right)\right)}{6\Lambda r^4}$$

$$F^{t}{}_{\theta,\theta,t} = \frac{\left(-2\Lambda^2 h_{\rm rr} + 9\Lambda h_{\theta\theta} + 27h_{\rm tt}\right)}{18r}$$

$$F^{t}{}_{\theta,\theta,r} = \frac{\left(\Lambda h_{\rm rr}{}^{(1,0,0)} - 9h_{\theta\theta}{}^{(1,0,0)} + 9h_{\rm t\theta}{}^{(0,1,0)}\right)}{2\Lambda r^4}$$

$$F^{t}{}_{\theta,\varphi,t} = \frac{\Lambda h_{\theta\varphi}}{2r}$$

$$F^{t}{}_{\theta,\varphi,r} = -\frac{9\left(h_{\theta\varphi}{}^{(1,0,0)} - h_{\rm t\varphi}{}^{(0,1,0)} + \cot(\theta)h_{\rm t\varphi}\right)}{2\Lambda r^4}$$

$$F^{t}{}_{\theta,\varphi,\theta} = -\frac{3h_{\rm t\varphi}}{2r}$$

$$F^{t}{}_{\varphi,r,t} = \frac{\left(\Lambda^2 h_{\rm rr}{}^{(0,0,1)} + 27\left(h_{\rm t\varphi}{}^{(1,0,0)} - h_{\rm tt}{}^{(0,0,1)}\right)\right)}{6\Lambda r^4}$$

$$F^{t}{}_{\varphi,\theta,t} = \frac{\Lambda h_{\theta\varphi}}{2r}$$

$$F^{t}{}_{\varphi,\theta,r} = -\frac{9\left(h_{\theta\varphi}{}^{(1,0,0)} - h_{\rm t\theta}{}^{(0,0,1)} + \cot(\theta)h_{\rm t\varphi}\right)}{2\Lambda r^4}$$

$$F^{t}{}_{\varphi,\varphi,t} = \frac{\left(-2\Lambda^2\sin^2(\theta)h_{\rm rr} + 9\Lambda h_{\varphi\varphi} + 27\sin^2(\theta)h_{\rm tt}\right)}{18r}$$

$$F^{t}{}_{\varphi,\varphi,r} = \frac{\left(\Lambda\sin^2(\theta)h_{\rm rr}{}^{(1,0,0)} - 9h_{\varphi\varphi}{}^{(1,0,0)} + 9\sin(\theta)\cos(\theta)h_{\rm t\theta} + 9h_{\rm t\varphi}{}^{(0,0,1)}\right)}{2\Lambda r^4}$$

$$F^{t}{}_{\varphi,\varphi,\theta} = \frac{3\sin^2(\theta)h_{\rm t\theta}}{2r}$$

$$F^{r}{}_{t,r,t} = -\frac{\left(\Lambda^3 h_{\mathrm{rr}} - 27\Lambda h_{\mathrm{tt}}\right)}{54r}$$
$$F^{r}{}_{t,\theta,t} = \frac{1}{54}\Lambda\left(\Lambda^2 h_{\mathrm{rr}}{}^{(0,1,0)} + 27\left(h_{\mathrm{t}\theta}{}^{(1,0,0)} - h_{\mathrm{tt}}{}^{(0,1,0)}\right)\right)$$
$$F^{r}{}_{t,\theta,r} = -\frac{\Lambda h_{\mathrm{t}\theta}}{2r}$$
$$F^{r}{}_{t,\varphi,t} = \frac{1}{54}\Lambda\left(\Lambda^2 h_{\mathrm{rr}}{}^{(0,0,1)} + 27\left(h_{\mathrm{t}\varphi}{}^{(1,0,0)} - h_{\mathrm{tt}}{}^{(0,0,1)}\right)\right)$$
$$F^{r}{}_{t,\varphi,r} = -\frac{\Lambda h_{\mathrm{t}\varphi}}{2r}$$
$$F^{r}{}_{t,\varphi,\theta} = -\frac{1}{2}\Lambda\left(h_{\mathrm{t}\theta}{}^{(0,0,1)} - h_{\mathrm{t}\varphi}{}^{(0,1,0)}\right)$$
$$F^{r}{}_{\theta,r,t} = \frac{\Lambda h_{\mathrm{t}\theta}}{2r}$$
$$F^{r}{}_{\theta,\theta,t} = -\frac{1}{18}\Lambda\left(\Lambda h_{\mathrm{rr}}{}^{(1,0,0)} - 9h_{\theta\theta}{}^{(1,0,0)} + 9h_{\mathrm{t}\theta}{}^{(0,1,0)}\right)$$
$$F^{r}{}_{\theta,\theta,r} = \frac{\Lambda\left(\Lambda h_{\mathrm{rr}} - 9h_{\theta\theta}\right)}{18r}$$
$$F^{r}{}_{\theta,\varphi,t} = \frac{1}{2}\Lambda\left(h_{\theta\varphi}{}^{(1,0,0)} - h_{\mathrm{t}\theta}{}^{(0,0,1)} + \cot(\theta)h_{\mathrm{t}\varphi}\right)$$
$$F^{r}{}_{\theta,\varphi,r} = -\frac{\Lambda h_{\theta\varphi}}{2r}$$
$$F^{r}{}_{\theta,\varphi,\theta} = \frac{1}{18}\Lambda\left(\Lambda h_{\mathrm{rr}}{}^{(0,0,1)} - 9h_{\theta\theta}{}^{(0,0,1)} + 9h_{\theta\varphi}{}^{(0,1,0)} + 9\cot(\theta)h_{\theta\varphi}\right)$$
$$F^{r}{}_{\varphi,r,t} = \frac{\Lambda h_{\mathrm{t}\varphi}}{2r}$$
$$F^{r}{}_{\varphi,\theta,t} = \frac{1}{2}\Lambda\left(h_{\theta\varphi}{}^{(1,0,0)} - h_{\mathrm{t}\varphi}{}^{(0,1,0)} + \cot(\theta)h_{\mathrm{t}\varphi}\right)$$
$$F^{r}{}_{\varphi,\theta,r} = -\frac{\Lambda h_{\theta\varphi}}{2r}$$
$$F^{r}{}_{\varphi,\varphi,t} = -\frac{1}{18}\Lambda\left(\Lambda\sin^2(\theta)h_{\mathrm{rr}}{}^{(1,0,0)} - 9h_{\varphi\varphi}{}^{(1,0,0)} + 9\sin(\theta)\cos(\theta)h_{\mathrm{t}\theta} + 9h_{\mathrm{t}\varphi}{}^{(0,0,1)}\right)$$
$$F^{r}{}_{\varphi,\varphi,r} = \frac{\Lambda\left(\Lambda\sin^2(\theta)h_{\mathrm{rr}} - 9h_{\varphi\varphi}\right)}{18r}$$
$$F^{r}{}_{\varphi,\varphi,\theta} = -\frac{1}{18}\Lambda\left(\Lambda\sin^2(\theta)h_{\mathrm{rr}}{}^{(0,1,0)} + 9\sin(\theta)\cos(\theta)h_{\theta\theta} + 9h_{\theta\varphi}{}^{(0,0,1)} - 9h_{\varphi\varphi}{}^{(0,1,0)} + 9\cot(\theta)h_{\varphi\varphi}\right)$$

$$F^{\theta}{}_{t,r,t} = -\frac{\left(\Lambda^2 h_{\mathrm{rr}}{}^{(0,1,0)} + 27\left(h_{\mathrm{t}\theta}{}^{(1,0,0)} - h_{\mathrm{tt}}{}^{(0,1,0)}\right)\right)}{18r^4}$$

$$F^{\theta}{}_{t,\theta,t} = \frac{\Lambda\left(2\Lambda^2 h_{\mathrm{rr}} - 9\left(\Lambda h_{\theta\theta} + 3h_{\mathrm{tt}}\right)\right)}{54r}$$

$$F^{\theta}{}_{t,\theta,r} = -\frac{\left(\Lambda h_{\mathrm{rr}}{}^{(1,0,0)} - 9h_{\theta\theta}{}^{(1,0,0)} + 9h_{\mathrm{t}\theta}{}^{(0,1,0)}\right)}{6r^4}$$

$$F^{\theta}{}_{t,\varphi,t} = -\frac{\Lambda^2 h_{\theta\varphi}}{6r}$$

$$F^{\theta}{}_{t,\varphi,r} = \frac{3\left(h_{\theta\varphi}{}^{(1,0,0)} - h_{\mathrm{t}\varphi}{}^{(0,1,0)} + \cot(\theta)h_{\mathrm{t}\varphi}\right)}{2r^4}$$

$$F^{\theta}{}_{t,\varphi,\theta} = \frac{\Lambda h_{\mathrm{t}\varphi}}{2r}$$

$$F^{\theta}{}_{r,r,t} = \frac{3h_{\mathrm{t}\theta}}{2r^5}$$

$$F^{\theta}{}_{r,\theta,t} = -\frac{\left(\Lambda h_{\mathrm{rr}}{}^{(1,0,0)} - 9h_{\theta\theta}{}^{(1,0,0)} + 9h_{\mathrm{t}\theta}{}^{(0,1,0)}\right)}{6r^4}$$

$$F^{\theta}{}_{r,\theta,r} = \frac{\left(\Lambda h_{\mathrm{rr}} - 9h_{\theta\theta}\right)}{6r^5}$$

$$F^{\theta}{}_{r,\varphi,t} = \frac{3\left(h_{\theta\varphi}{}^{(1,0,0)} - h_{\mathrm{t}\theta}{}^{(0,0,1)} + \cot(\theta)h_{\mathrm{t}\varphi}\right)}{2r^4}$$

$$F^{\theta}{}_{r,\varphi,r} = -\frac{3h_{\theta\varphi}}{2r^5}$$

$$F^{\theta}{}_{r,\varphi,\theta} = \frac{\left(\Lambda h_{\mathrm{rr}}{}^{(0,0,1)} - 9h_{\theta\theta}{}^{(0,0,1)} + 9h_{\theta\varphi}{}^{(0,1,0)} + 9\cot(\theta)h_{\theta\varphi}\right)}{6r^4}$$

$$F^{\theta}{}_{\varphi,r,t} = -\frac{3\left(h_{\mathrm{t}\theta}{}^{(0,0,1)} - h_{\mathrm{t}\varphi}{}^{(0,1,0)}\right)}{2r^4}$$

$$F^{\theta}{}_{\varphi,\theta,t} = -\frac{\Lambda h_{\mathrm{t}\varphi}}{2r}$$

$$F^{\theta}{}_{\varphi,\theta,r} = -\frac{\left(\Lambda h_{\mathrm{rr}}{}^{(0,0,1)} - 9h_{\theta\theta}{}^{(0,0,1)} + 9h_{\theta\varphi}{}^{(0,1,0)} + 9\cot(\theta)h_{\theta\varphi}\right)}{6r^4}$$

$$F^{\theta}{}_{\varphi,\varphi,t} = \frac{\Lambda\sin^2(\theta)h_{\mathrm{t}\theta}}{2r}$$

$$F^{\theta}{}_{\varphi,\varphi,r} = \frac{\left(\Lambda\sin^2(\theta)h_{\mathrm{rr}}{}^{(0,1,0)} + 9\sin(\theta)\cos(\theta)h_{\theta\theta} + 9h_{\theta\varphi}{}^{(0,0,1)} - 9h_{\varphi\varphi}{}^{(0,1,0)} + 9\cot(\theta)h_{\varphi\varphi}\right)}{6r^4}$$

$$F^{\theta}{}_{\varphi,\varphi,\theta} = \frac{\Lambda\left(9\left(\sin^2(\theta)h_{\theta\theta} + h_{\varphi\varphi}\right) - 2\Lambda\sin^2(\theta)h_{\mathrm{rr}}\right)}{18r}$$

$$F^{\varphi}{}_{t,r,t} = -\frac{\csc^2(\theta)\left(\Lambda^2 h_{\mathrm{rr}}{}^{(0,0,1)} + 27\left(h_{\mathrm{t}\varphi}{}^{(1,0,0)} - h_{\mathrm{tt}}{}^{(0,0,1)}\right)\right)}{18r^4}$$

$$F^{\varphi}{}_{t,\theta,t} = -\frac{\Lambda^2\csc^2(\theta)h_{\theta\varphi}}{6r}$$

$$F^{\varphi}{}_{t,\theta,r} = \frac{3\csc^2(\theta)\left(h_{\theta\varphi}{}^{(1,0,0)} - h_{\mathrm{t}\theta}{}^{(0,0,1)} + \cot(\theta)h_{\mathrm{t}\varphi}\right)}{2r^4}$$

$$F^{\varphi}{}_{t,\varphi,t} = \frac{\Lambda\left(2\Lambda^2 h_{\mathrm{rr}} - 9\left(\Lambda\csc^2(\theta)h_{\varphi\varphi} + 3h_{\mathrm{tt}}\right)\right)}{54r}$$

$$F^{\varphi}{}_{t,\varphi,r} = -\frac{\left(\Lambda h_{\mathrm{rr}}{}^{(1,0,0)} - 9\csc^2(\theta)h_{\varphi\varphi}{}^{(1,0,0)} + 9\cot(\theta)h_{\mathrm{t}\theta} + 9\csc^2(\theta)h_{\mathrm{t}\varphi}{}^{(0,0,1)}\right)}{6r^4}$$

$$F^{\varphi}{}_{t,\varphi,\theta} = -\frac{\Lambda h_{\mathrm{t}\theta}}{2r}$$

$$F^{\varphi}{}_{r,r,t} = \frac{3\csc^2(\theta)h_{\mathrm{t}\varphi}}{2r^5}$$

$$F^{\varphi}{}_{r,\theta,t} = \frac{3\csc^2(\theta)\left(h_{\theta\varphi}{}^{(1,0,0)} - h_{\mathrm{t}\varphi}{}^{(0,1,0)} + \cot(\theta)h_{\mathrm{t}\varphi}\right)}{2r^4}$$

$$F^{\varphi}{}_{r,\theta,r} = -\frac{3\csc^2(\theta)h_{\theta\varphi}}{2r^5}$$

$$F^{\varphi}{}_{r,\varphi,t} = -\frac{\left(\Lambda h_{\mathrm{rr}}{}^{(1,0,0)} - 9\csc^2(\theta)h_{\varphi\varphi}{}^{(1,0,0)} + 9\cot(\theta)h_{\mathrm{t}\theta} + 9\csc^2(\theta)h_{\mathrm{t}\varphi}{}^{(0,0,1)}\right)}{6r^4}$$

$$F^{\varphi}{}_{r,\varphi,r} = \frac{\left(\Lambda h_{\mathrm{rr}} - 9\csc^2(\theta)h_{\varphi\varphi}\right)}{6r^5}$$

$$F^{\varphi}{}_{r,\varphi,\theta} = -\frac{\left(\Lambda h_{\mathrm{rr}}{}^{(0,1,0)} + 9\cot(\theta)h_{\theta\theta} + 9\csc^2(\theta)h_{\theta\varphi}{}^{(0,0,1)} - 9\csc^2(\theta)h_{\varphi\varphi}{}^{(0,1,0)} + 9\cot(\theta)\csc^2(\theta)h_{\varphi\varphi}\right)}{6r^4}$$

$$F^{\varphi}{}_{\theta,r,t} = \frac{3\csc^2(\theta)\left(h_{\mathrm{t}\theta}{}^{(0,0,1)} - h_{\mathrm{t}\varphi}{}^{(0,1,0)}\right)}{2r^4}$$

$$F^{\varphi}{}_{\theta,\theta,t} = \frac{\Lambda\csc^2(\theta)h_{\mathrm{t}\varphi}}{2r}$$

$$F^{\varphi}{}_{\theta,\theta,r} = \frac{\csc^2(\theta)\left(\Lambda h_{\mathrm{rr}}{}^{(0,0,1)} - 9h_{\theta\theta}{}^{(0,0,1)} + 9h_{\theta\varphi}{}^{(0,1,0)} + 9\cot(\theta)h_{\theta\varphi}\right)}{6r^4}$$

$$F^{\varphi}{}_{\theta,\varphi,t} = -\frac{\Lambda h_{\mathrm{t}\theta}}{2r}$$

$$F^{\varphi}{}_{\theta,\varphi,r} = -\frac{\left(\Lambda h_{\mathrm{rr}}{}^{(0,1,0)} + 9\cot(\theta)h_{\theta\theta} + 9\csc^2(\theta)h_{\theta\varphi}{}^{(0,0,1)} - 9\csc^2(\theta)h_{\varphi\varphi}{}^{(0,1,0)} + 9\cot(\theta)\csc^2(\theta)h_{\varphi\varphi}\right)}{6r^4}$$

$$F^{\varphi}{}_{\theta,\varphi,\theta} = \frac{\Lambda\left(2\Lambda h_{\mathrm{rr}} - 9\left(h_{\theta\theta} + \csc^2(\theta)h_{\varphi\varphi}\right)\right)}{18r}$$

Note that all $h_{\mu\nu}$ functions above are $[t,\theta,\phi]$ dependent, while $r$ dependency is given explicitly. Functions $f^{(1,0,0)}, f^{(0,1,0)}, f^{(0,0,1)}$ mean $\frac{\partial f}{\partial t}, \frac{\partial f}{\partial \theta}, \frac{\partial f}{\partial \phi}$, respectively.

## 4 Asymptotic Einstein tensor

The Einstein equations decompose accordingly to $0 = G_{\mu\nu} = \bar{G}_{\mu\nu} + G^{(1)}_{\mu\nu}$. The AdS part of Einstein tensor is identically vanishing, and the rest of components correspond to

$$
\begin{aligned}
G^{(1)}_{tt} &= \frac{\Lambda}{6r}\left(\frac{\Lambda^2}{3}h_{rr} - 3h_{tt} - \Lambda\left(h_{\theta\theta} + \csc^2\theta h_{\varphi\varphi}\right)\right) \\
G^{(1)}_{tr} &= -\frac{3}{2r^4}\left(\frac{2\Lambda}{9}\partial_t h_{rr} - \partial_t h_{\theta\theta} + \partial_\theta h_{t\theta} + \cot\theta h_{t\theta} - \csc^2\theta\partial_t h_{\varphi\varphi} + \csc^2\theta\partial_\varphi h_{t\varphi}\right) \\
G^{(1)}_{t\theta} &= \frac{1}{2r^3}\Big(\frac{2\Lambda}{3}\partial_t h_{r\theta} + \frac{\Lambda}{3}\partial_t\partial_\theta h_{rr} - 2h_{t\theta} + \frac{2}{3}\Lambda\partial_\theta h_{tr} + \cot\theta\partial_t h_{\theta\theta} \\
&+ \csc^2\theta\left(\partial_t\partial_\varphi h_{\theta\varphi} - \partial_t\partial_\theta h_{\varphi\varphi} + \cot\theta\partial_t h_{\varphi\varphi} - \partial^2_\varphi h_{t\theta} + \partial_\theta\partial_\varphi h_{t\varphi}\right)\Big) \\
G^{(1)}_{t\varphi} &= \frac{1}{6r^3}\Big(\Lambda\partial_t\partial_\varphi h_{rr} + 2\Lambda\partial_t h_{r\varphi} - 3\partial_t\partial_\varphi h_{\theta\theta} + 3\partial_t\partial_\theta h_{\theta\varphi} + 3\cot\theta\partial_t h_{\theta\varphi} \\
&+ 3\partial_\theta\partial_\varphi h_{t\theta} - 3\cot\theta\partial_\varphi h_{t\theta} + 2\Lambda\partial_\varphi h_{tr} - 6h_{t\varphi} - 3\partial^2_\theta h_{t\varphi} + 3\cot(\theta)\partial_\theta h_{t\varphi}\Big) \\
G^{(1)}_{rr} &= \frac{3}{2\Lambda r^5}\left(\frac{\Lambda^2}{3}h_{rr} - 3h_{tt} - \Lambda\left(h_{\theta\theta} + \csc^2\theta h_{\varphi\varphi}\right)\right) \\
G^{(1)}_{r\theta} &= -\frac{3}{2\Lambda r^4}\Big(\frac{2\Lambda^2}{9}\partial_\theta h_{rr} + 3\partial_t h_{t\theta} - 3\partial_\theta h_{tt} + \Lambda\cot\theta h_{\theta\theta} + \Lambda\cot(\theta)\csc^2\theta h_{\varphi\varphi} \\
&+ \Lambda\csc^2\theta\partial_\varphi h_{\theta\varphi} - \Lambda\csc^2\theta\partial_\theta h_{\varphi\varphi}\Big) \\
G^{(1)}_{r\varphi} &= -\frac{1}{6\Lambda r^4}\left(2\Lambda^2\partial_\varphi h_{rr} - 9\Lambda\partial_\varphi h_{\theta\theta} + 9\Lambda\partial_\theta h_{\theta\varphi} + 9\Lambda\cot\theta h_{\theta\varphi} - 27\partial_\varphi h_{tt} + 27\partial_t h_{t\varphi}\right) \\
G^{(1)}_{\theta\theta} &= \frac{1}{2r}\left(\frac{\Lambda^2}{3}h_{rr} - 3h_{tt} - \Lambda\left(h_{\theta\theta} + \csc^2\theta h_{\varphi\varphi}\right)\right) \\
G^{(1)}_{\theta\varphi} &= \frac{1}{6\Lambda r^3}\Big(2\Lambda^2\partial_\varphi h_{r\theta} + \Lambda^2\partial_\theta\partial_\varphi h_{rr} + 2\Lambda^2\partial_\theta h_{r\varphi} - 18\Lambda h_{\theta\varphi} \\
&- 9\partial^2_t h_{\theta\varphi} + 9\partial_t\partial_\varphi h_{t\theta} - 9\partial_\theta\partial_\varphi h_{tt} + 9\partial_t\partial_\theta h_{t\varphi} \\
&- \Lambda^2\cot\theta\partial_\varphi h_{rr} - 4\Lambda^2\cot\theta h_{r\varphi} + 9\cot\theta\partial_\varphi h_{tt} - 18\cot\theta\partial_t h_{t\varphi}\Big) \\
G^{(1)}_{\varphi\varphi} &= \frac{1}{2r}\sin^2\theta\left(\frac{\Lambda^2}{3}h_{rr} - 3h_{tt} - \Lambda\left(h_{\theta\theta} + \csc^2\theta h_{\varphi\varphi}\right)\right) .
\end{aligned}
$$
